# Supplementary material for: Sketch-Driven Regular Expression Generation from Natural Language and Examples
Source: arXiv:1908.05848 source file (2020-08-03)
Supplement: Supplementary file 1 [file appendix.tex]

\newpage
\section*{Appendix A: Regex Language}

\begin{figure}[h]
  \small
   \scalebox{.50}{
  \begin{tabular}{|c|c|c|}
  \hline
  \multicolumn{3}{|c|}{Non-terminals $\prog$} \\
  \hline
     $\texttt{StartsWith}(\prog) \rightarrow \prog.*$  & $\texttt{EndsWith}(\prog) \rightarrow .*\prog$ & $\texttt{Contains}(\prog) \rightarrow .*\prog.*$ \\
  \hline
      $\texttt{Not}(\prog) \rightarrow  {\raise.17ex\hbox{$\scriptstyle\sim$}} \prog$ & $\texttt{Optional}(\prog) \rightarrow \prog \texttt{?}$ & 
      $\texttt{KleeneStar}(\prog) \rightarrow \prog*$ \\
  \hline
      $\texttt{Concat}(\prog_1, \prog_2) \rightarrow \prog_1 \prog_2$ &
      $\texttt{And}(\prog_1, \prog_2) \rightarrow \prog_1 \texttt{\&}  \prog_2$ &
      $\texttt{Or}(\prog_1, \prog_2) \rightarrow \prog_1 \texttt{|} \prog_2$ \\
  \hline
      $\texttt{Repeat}(\prog, k) \rightarrow \prog\{k\}$ &
      $\texttt{RepeatAtLeast}(\prog, k) \rightarrow \prog\{k,\}$ &
      $\texttt{RepeatRange}(\prog, k_1, k_2) \rightarrow \prog\{k_1, k_2\}$ \\
  \hline
  \end{tabular}}
  
  \scalebox{.50}{
  \begin{tabular}{|c|c|c|c|}
  \hline
  \multicolumn{4}{|c|}{Terminals} \\
  \hline
  $\texttt{<let>} \rightarrow \texttt{[A-Za-z]}$ &
  $\texttt{<vow>} \rightarrow \texttt{[AEIOUaeiou]}$ &
  $\texttt{<cap>} \rightarrow \texttt{[A-Z]}$ &
  $\texttt{<low>} \rightarrow \texttt{[a-z]}$ \\
  \hline
  $\texttt{<num>} \rightarrow \texttt{[0-9]}$ & 
  $\texttt{<alphanum>} \rightarrow \texttt{[A-Za-z0-9]}$ & 
  \multicolumn{2}{|c|}{$\texttt{<any>} \rightarrow \texttt{.}$} \\
  \hline
  \multicolumn{2}{|c|}{$\texttt{<eps>} \rightarrow \epsilon$} &
  \multicolumn{2}{|c|}{$\texttt{<null>} \rightarrow \emptyset$} \\
  \hline
  \end{tabular}}
  
  % \vspace{-10pt}
  \caption{Our regex language ($k$ is a positive integer). The right arrow $\rightarrow$ shows how to translate our language to a standard regular expression language.}
  \figlabel{dslsyntax}
  \end{figure}
 
\section*{Appendix B: Hyperparameters Of Our Neural Model}
% Recall that the architecture used in \textsc{DeepRegex (Ours)} and \textsc{DeepSketch} consists of an input embedding layer, a bidirectional LSTM encoder, an output embedding layer, and a unidirectional decoder. For the hyperparameters, the dimension of both the input embedding layer and the output embedding layer is 128. 
% The original \textsc{DeepRegex} model uses a.
\begin{table}[h]
    \centering
    \small
    \begin{tabular}{l|c|c}
    \toprule
        & Ours & \citet{deepregex}  \\
    \midrule
 input dim  &128 & 64 \\
    encoder type & BiLSTM & LSTM \\
    encoder layer & 1 & 2\\
    encoder size & 256 & 512\\
 output dim   &128 & 64 \\
    decoder type & LSTM & LSTM \\
    decoder layer & 1 & 2\\
    decoder size & 256 & 512\\
    \bottomrule
         
    \end{tabular}
    \caption{Comparison of the neural model used in our approach and the original model used in \textsc{DeepRegex}\cite{deepregex}. We use a single layer BiLSTM encoder and a single layer LSTM decoder while original \textsc{DeepRegex} uses a double-layer LSTM encoder and a double-layer LSTM decoder.}
    \label{tab:my_label}
\end{table}
\onecolumn
\section*{Appendix C: Grammar}
\footnotesize
\subsection{Notes about the parsing rules}
Recall from the paper that we specify our grammar using rules of the following form: $\alpha_1 ... \alpha_n \rightarrow  c[\beta]  $.

The $\beta$ can be exactly the target derivation, or a semantic function (such as \text{IdentityFn}, \text{SelectFn}, \text{sketch.UnarySketchFn} etc.) that is applied to produce target derivation with arguments. 

There are two types of arguments: 
\begin{itemize}
    \item \text{arg:i} represents selecting the $i^{th}$ position from the matched $\alpha_1 ... \alpha_n$ and passing it to the function. For example, the rule $  (\text{\$Skip } \text{\$SKETCH} \rightarrow \text{\$ROOT }[\text{SelectFn arg:1}])$ selects the first category from the source sequence, which is the $\text{\$SKETCH}$ (Notes that Sempre starts indexing from 0).
    \item \text{val:n} represents passing the integer value $n$ to the function. For example, the rule \\ $(\text{\$CC1 \$MARKER\_ONLY} \rightarrow  \text{\$PROGRAM}[\text{sketch.RepeatatleastFn arg:0, val:1}])$ passes the first category in the matched source sequence \text{\$MARKER\_ONLY} and the integer value $1$ to the semantic function \text{sketch.RepeatatleastFn}.
    
\end{itemize}

\subsection{Compositional Rules}
\quad\ \textbf{Root}

$\text{\$Sketch} \rightarrow \text{\$ROOT [IdentityFn arg:0]}$

$\text{\$Skip \$SKETCH} \rightarrow \text{\$ROOT [SelectFn arg:1]}$

\hspace{0.5cm}

\textbf{Skip tokens rule}

$\text{\$LEMMA\_PHRASE} \rightarrow \text{\$Skip [ConstantFn arg:null]}$

\hspace{0.5cm}

\textbf{Parse a number}

$\text{\$LEMMA\_PHRASE} \rightarrow \text{\$INT1 [NumberFn val:NUMBER]}$

\hspace{0.5cm}

\textbf{Parse a character class or constant to a regex}

$\text{\$CC} \rightarrow \text{\$PROGRAM [IdentifyFn arg:0]}$

$\text{\$CONST} \rightarrow \text{\$PROGRAM [IdentifyFn arg:0]}$

\hspace{0.5cm}

\textbf{Hierarchical sketch parse rules}

$\text{\$LIST\_PROGRAM} \rightarrow \text{\$SKETCH [sketch.UnarySketchFn arg:0]}$

$\text{\$PROGRAM} \rightarrow \text{\$LIST\_PROGRAM [IdentityFn arg:0]}$

$\text{\$PROGRAM \$LIST\_PROGRAM} \rightarrow \text{\$LIST\_PROGRAM [sketch.SketchJoinFn arg:0]}$

\hspace{0.5cm}

\textbf{Operator: NotContain}

$\text{\$MARKER\_NOTCONTAIN \$SKETCH} \rightarrow \text{\$SKETCH [sketch.NotContainFn arg:1]}$

$\text{\$MARKER\_NOTCONTAIN \$PROGRAM} \rightarrow \text{\$PROGRAM [sketch.NotContainFn arg:1]}$

\hspace{0.5cm}

\textbf{Operator: Not}

$\text{\$MARKER\_NOT \$SKETCH} \rightarrow \text{\$SKETCH [sketch.NotFn arg:1]}$

$\text{\$MARKER\_NOT \$PROGRAM} \rightarrow \text{\$PROGRAM [sketch.NotFn arg:1]}$

$\text{\$MARKER\_NON1 \$CONST} \rightarrow \text{\$PROGRAM [sketch.NotccFn arg:1]}$

\hspace{0.5cm}

\textbf{Operator: Optional}

$\text{\$MARKER\_NOT \$CC} \rightarrow \text{\$PROGRAM [sketch.OptionalFn arg:1]}$

\hspace{0.5cm}

\textbf{Operator: StartWith, EndWith}

$\text{\$MARKER\_STARTWITH \$PROGRAM} \rightarrow \text{\$PROGRAM [sketch.StartwithFn arg:1]}$

$\text{\$MARKER\_ENDWITH \$PROGRAM} \rightarrow \text{\$PROGRAM [sketch.EndwithFn arg:1]}$

$\text{\$PROGRAM \$MARKER\_ATEND } \rightarrow \text{\$PROGRAM [sketch.EndwithFn arg:0]}$

\hspace{0.5cm}

\textbf{Operator: Concat}

$\text{\$PROGRAM \$MARKER\_CONCAT \$PROGRAM} \rightarrow \text{\$PROGRAM [sketch.ConcatFn arg:0, arg:2]}$

$\text{\$PROGRAM \$MARKER\_CONCAT \$SKETCH} \rightarrow \text{\$SKETCH [sketch.ConcatFn arg:0, arg:2]}$

$\text{\$SKETCH \$MARKER\_CONCAT \$PROGRAM} \rightarrow \text{\$SKETCH [sketch.ConcatFn arg:0, arg:2]}$

$\text{\$SKETCH \$MARKER\_CONCAT \$SKETCH} \rightarrow \text{\$SKETCH [sketch.ConcatFn arg:0, arg:2]}$

$\text{\$PROGRAM \$MARKER\_FOLLOW \$PROGRAM} \rightarrow \text{\$PROGRAM [sketch.ConcatFn arg:2, arg:0]}$

$\text{\$PROGRAM \$MARKER\_FOLLOW \$SKETCH} \rightarrow \text{\$SKETCH [sketch.ConcatFn arg:2, arg:0]}$

$\text{\$SKETCH \$MARKER\_FOLLOW \$PROGRAM} \rightarrow \text{\$SKETCH [sketch.ConcatFn arg:2, arg:0]}$

$\text{\$SKETCH \$MARKER\_FOLLOW \$SKETCH} \rightarrow \text{\$SKETCH [sketch.ConcatFn arg:2, arg:0]}$

\hspace{0.5cm}

\textbf{Operator: Repeat}

$\text{\$INT \$CC} \rightarrow \text{\$PROGRAM [sketch.RepeatFn arg:1, arg:0]}$

$\text{\$CC \$MARKER\_LENGTH \$INT} \rightarrow \text{\$PROGRAM [sketch.RepeatFn arg:0, arg:2]}$

$\text{\$MARKER\_LENGTH \$INT \$CC} \rightarrow \text{\$PROGRAM [sketch.RepeatFn arg:2, arg:1]}$

$\text{\$INT1 \$MARKER\_OR1 \$INT1 \$CC} \rightarrow \text{\$PROGRAM [sketch.RepeatAOrBFn arg:3, arg:0, arg:2]}$

\hspace{0.5cm}

\textbf{Operator: RepeatAtLeast}

$\text{\$MARKER\_ONLY1 \$CC} \rightarrow \text{\$PROGRAM [sketch.RepeatatleastFn arg:1, val:1]}$

$\text{\$CC1 \$MARKER\_ONLY} \rightarrow \text{\$PROGRAM [sketch.RepeatatleastFn arg:0, val:1]}$

$\text{\$INT1 \$MARKER\_ORMORE1 \$CC} \rightarrow \text{\$PROGRAM [sketch.RepeatatleastFn arg:2, arg:0]}$

$\text{\$PROGRAM \$INT1 \$MARKER\_ORMORE1} \rightarrow \text{\$PROGRAM [sketch.RepeatatleastFn arg:0, arg:1]}$

\hspace{0.5cm}

\textbf{Operator: RepeatRange}

$\text{\$MARKER\_ATMAX1 \$INT \$CC} \rightarrow \text{\$PROGRAM [sketch.RepeatrangeFn arg:2, val:1, arg:1]}$

$\text{\$MARKER\_ATMAX \$INT \$CC} \rightarrow \text{\$PROGRAM [sketch.RepeatrangeFn arg:2, val:1, arg:1]}$

$\text{\$INT \$CC} \rightarrow \text{\$PROGRAM [sketch.RepeatrangeFn arg:1, val:1, arg:0]}$

\hspace{0.5cm}

\textbf{Extract constants}

$\text{\$CONST\_SET} \rightarrow \text{\$CC1 [IdentityFn arg:0]}$

$\text{\$CONST1}\ \text {\$CONST\_SET} \rightarrow \text{\$CONST\_SET [sketch.ConstUnionFn arg:0, arg:1]}$

$\text{\$CONST1 \$CONST1} \rightarrow \text{\$CONST\_SET [sketch.ConstUnionFn arg:0, arg:1]}$

$\text{\$CONST1 \$MAKRKER\_CONSTSETUNION1 \$CONST1} \rightarrow \text{\$CONST\_SET [sketch.ConstUnionFn arg:0, arg:2]}$

$\text{\$CONST1 \$MAKRKER\_CONSTSETUNION1 \$CONST\_SET} \rightarrow \text{\$CONST\_SET [sketch.ConstUnionFn arg:0, arg:2]}$

$\text{\$CCPHRASE1 \$MAKRKER\_CONSTSETUNION1 \$CONST1} \rightarrow \text{\$CONST\_SET [sketch.ConstUnionFn arg:0, arg:2]}$

$\text{\$CCPHRASE1 \$MAKRKER\_CONSTSETUNION1 \$CCPHRASE1} \rightarrow \text{\$CONST\_SET [sketch.ConstUnionFn arg:0, arg:2]}$

$\text{\$CCPHRASE1 \$MAKRKER\_CONSTSETUNION1 \$CONST\_SET} \rightarrow \text{\$CONST\_SET [sketch.ConstUnionFn arg:0, arg:2]}$

$\text{`` \$PHRASE ''} \rightarrow \text{\$CONST1 [sketch.ConstFn arg:0]}$

\hspace{0.5cm}

\textbf{``Separated/Split by''}

$\text{\$SKETCH \$PROGRAM \$MARKER\_SEP} \rightarrow \text{\$SKETCH [sketch.SepFn arg:0,arg:1]}$

$\text{\$PROGRAM \$PROGRAM \$MARKER\_SEP} \rightarrow \text{\$PROGRAM [sketch.SepFn arg:0,arg:1]}$

$\text{\$PROGRAM \$MARKER\_BETWEEN \$SKETCH} \rightarrow \text{\$SKETCH [sketch.SepFn arg:2,arg:0]}$

$\text{\$PROGRAM \$MARKER\_BETWEEN \$PROGRAM} \rightarrow \text{\$PROGRAM [sketch.SepFn arg:2,arg:0]}$

$\text{\$SKETCH \$MARKER\_SPLITBY \$PROGRAM} \rightarrow \text{\$SKETCH [sketch.SepFn arg:0,arg:2]}$

\hspace{0.5cm}

\textbf{``Decimal''}

$\text{\$PROGRAM \$MARKER\_DECIMAL \$PROGRAM} \rightarrow \text{\$SKETCH [sketch.DecimalFn arg:0, arg:2]}$

$\text{\$MARKER\_DECIMAL \$PROGRAM \$PROGRAM} \rightarrow \text{\$SKETCH [sketch.DecimalFn arg:1, arg:2]}$

$\text{\$PROGRAM \$PROGRAM \$MARKER\_DECIMAL} \rightarrow \text{\$SKETCH [sketch.DecimalFn arg:0, arg:1]}$

$\text{\$MARKER\_DECIMALNUM} \rightarrow \text{\$SKETCH [sketch.DecimalFn]}$

\hspace{0.5cm}

\textbf{Skip Rules: we present one example here as a skip rule that is required by Sempre to allow skipping tokens when matching compositional rules. These rules can be generated automatically and hence we don't count these as part of the compositional rules. }

$\text{\$Skip optional} \rightarrow \text{\$CC [SelectFn arg:0]}$

\hspace{0.5cm}

\textbf{Lexicon mapping rules: we present one example here that matches lexicons in the lexicon files to base-case target category to allow compositional rules build up on lexicons. These rules can be generated automatically and hence we don't count these as part of the compositional rules.}

$\text{\$CCPHRASE1} \rightarrow \text{\$CC1 [IdentityFn arg:0]}$
\subsection{Lexical Rules}

\quad\ $\text{number} \rightarrow \text{\$CC\ [<num>]}$

$\text{numeric} \rightarrow \text{\$CC    [<num>]}$

$\text{numeral} \rightarrow \text{\$CC    [<num>]}$

$\text{decimal} \rightarrow \text{\$CC [<num>]}$

$\text{digit} \rightarrow \text{\$CC [<num>]}$

$\text{alphanumeric} \rightarrow \text{\$CC [<alphanum>]}$

$\text{hexadecimal} \rightarrow \text{\$CC [<hex>]}$

$\text{string} \rightarrow \text{\$CC [<any>]}$

$\text{character} \rightarrow \text{\$CC [<let>]}$

$\text{letter} \rightarrow \text{\$CC [<let>]}$

$\text{word} \rightarrow \text{\$CC [<let>]}$

$\text{alphabet} \rightarrow \text{\$CC [<let>]}$

$\text{lower case letter} \rightarrow \text{\$CC [<low>]}$

$\text{small letter} \rightarrow \text{\$CC [<low>]}$

$\text{upper case letter} \rightarrow \text{\$CC [<cap>]}$

$\text{capital letter} \rightarrow \text{\$CC [<cap>]}$

$\text{vowel} \rightarrow \text{\$CC [<vow>]}$

$\text{special character} \rightarrow \text{\$CC [<spec>]}$

$\text{special char} \rightarrow \text{\$CC [<spec>]}$

$\text{comma} \rightarrow \text{\$CONST [<,>]}$

$\text{colon} \rightarrow \text{\$CONST [<:>]}$

$\text{semicolon} \rightarrow \text{\$CONST [<;>]}$

$\text{space} \rightarrow \text{\$CONST [<space>]}$

$\text{underscore} \rightarrow \text{\$CONST [<\_>]}$

$\text{dash} \rightarrow \text{\$CONST [<->]}$

$\text{percentage sign} \rightarrow \text{\$CONST [<\%>]}$

$\text{percentage sign} \rightarrow \text{\$CONST [<\%>]}$

$\text{not} \rightarrow \text{\$OP.NOT [op.not]}$

$\text{non} \rightarrow \text{\$OP.NON [op.non]}$

$\text{or} \rightarrow \text{\$OP.OR [op.or]}$

$\text{optional} \rightarrow \text{\$OP.OPTIONAL [op.optional]}$

$\text{not contain} \rightarrow \text{\$OP.NOTCONTAIN [op.notcontain]}$

$\text{not allow} \rightarrow \text{\$OP.NOTCONTAIN [op.notcontain]}$

$\text{or more} \rightarrow \text{\$OP.ORMORE [op.ormore]}$

$\text{or more time} \rightarrow \text{\$OP.ORMORE [op.ormore]}$

$\text{max} \rightarrow \text{\$OP.MAX [op.max]}$

$\text{decimal} \rightarrow \text{\$OP.DECIMAL [op.decimal]}$

$\text{double number} \rightarrow \text{\$OP.DECIMALNUM [op.decimalnum]}$

$\text{length} \rightarrow \text{\$OP.LENGTH [op.length]}$

$\text{,} \rightarrow \text{\$OP.CONSTSETUNION [op.constsetunion]}$

$\text{(, optional) or} \rightarrow \text{\$OP.CONSTSETUNION [op.constsetunion]}$

$\text{(, optional) and} \rightarrow \text{\$OP.CONSTSETUNION [op.constsetunion]}$

$\text{separate} \rightarrow \text{\$OP.SEP [op.sep]}$

$\text{delimit} \rightarrow \text{\$OP.SEP [op.sep]}$

$\text{between} \rightarrow \text{\$OP.BETWEEN [op.between]}$

$\text{separated} \rightarrow \text{\$OP.BETWEEN [op.between]}$

$\text{split by} \rightarrow \text{\$OP.SPLITBY [op.splitby]}$

$\text{divide by} \rightarrow \text{\$OP.SPLITBY [op.splitby]}$

$\text{end with} \rightarrow \text{\$OP.ENDWITH [op.endwith]}$

$\text{finish with} \rightarrow \text{\$OP.ENDWITH [op.endwith]}$

$\text{end in} \rightarrow \text{\$OP.ENDWITH [op.endwith]}$

$\text{terminate} \rightarrow \text{\$OP.ENDWITH [op.endwith]}$

$\text{at end} \rightarrow \text{\$OP.ATEND [op.atend]}$

$\text{start with} \rightarrow \text{\$OP.STARTWITH [op.startwith]}$

$\text{start in} \rightarrow \text{\$OP.STARTWITH [op.startwith]}$

$\text{at the begin} \rightarrow \text{\$OP.STARTWITH [op.startwith]}$

$\text{before} \rightarrow \text{\$OP.CONCAT [op.concat]}$

$\text{follow by} \rightarrow \text{\$OP.CONCAT [op.concat]}$

$\text{next} \rightarrow \text{\$OP.CONCAT [op.concat]}$

$\text{then} \rightarrow \text{\$OP.CONCAT [op.concat]}$

$\text{prior to} \rightarrow \text{\$OP.CONCAT [op.concat]}$

$\text{precede} \rightarrow \text{\$OP.CONCAT [op.concat]}$

$\text{after} \rightarrow \text{\$OP.FOLLOW [op.follow]}$

$\text{bulletpoint} \rightarrow \text{\$OP.FOLLOW [op.follow]}$

$\text{up to} \rightarrow \text{\$OP.ATMAX [op.atmax]}$

$\text{at max} \rightarrow \text{\$OP.ATMAX [op.atmax]}$

$\text{only} \rightarrow \text{\$OP.ONLY [op.only]}$
